# Supplementary material for: Local Implicit Normalizing Flow for Arbitrary-Scale Image Super-Resolution
Source: arXiv:2303.05156 source file (2023-07-13)
Supplement: Supplementary file 1 [file all.tex]

\section{Anonymous GitHub Link}
\label{sec::github}
The anonymous GitHub link of our project:  \url{https://anonymous.4open.science/r/LINF-1674}

\section{Notation Table}
\label{sec::notation}
The symbols used in this paper are summarized in Table~\ref{tab:supp:notation}.

\section{Background}
\label{sec::background}
% \subsection{Normalizing Flow} 
% \label{subsec:nf}

% In this section, we introduce background knowledge of implicit neural representation to make our paper self-contained.
In this section, we briefly review the essential background knowledge of implicit neural representation to allow the presentation of this work self-contained.

\subsection{Implicit Neural Representation} 
\label{subsec:inr}
Implicit neural representation parametrized by multilayer perceptron (MLP) approximates complex signals by mapping input coordinates to output values. Compared to classic discrete representation (e.g., pixels for 2D images and point clouds, meshes, and voxel grids for 3D objects), Such coordinate-based MLP successfully represents the signals in the continuous domain. Recent works have achieved promising results in modeling 2D images~\cite{siren, liif} and 3D geometry and appearance~\cite{imnet, Occupancy_Networks, deepsdf, srn, nerf}.
However, many previous works focus on fitting the signal of a single instance, e.g., an image~\cite{siren} or a scene~\cite{nerf}. To make implicit neural representation generalize to unseen data, latent vector conditioning~\cite{Occupancy_Networks, deepsdf} and hypernetwork setting~\cite{srn, siren} have been proposed. The former fed the latent vector corresponding to a particular instance along with coordinates to the MLP network, and the latter used a hypernetwork to map a latent to the weights of MLP. 
Our work is based on the idea of local implicit neural representation~\cite{jiang2020lig, liif}. Instead of taking a global latent as a condition, local implicit neural representation captures the localized details by conditioning on a local feature.

\section{Detailed Experiment}
\label{sec::experiment}
\subsection{Analysis on the Patch Size} 
\label{subsec:patch}
\begin{table}[t]

\newcommand{\mytoprule}{\toprule[1.2pt]}
\centering
\footnotesize
\resizebox{0.8\columnwidth}{!}{%
    \begin{tabular}{l|c|c|c}
        \hline
        Method & PSNR$\uparrow$ & SSIM$\uparrow$ & LPIPS$\downarrow$ \\
        \hline
        \hline
        n = 1 (pixel) & 27.94 & 0.79 & 0.174 \\
        n = 3 (3$\times$3 patch) & 27.43 & 0.77 & 0.158 \\
        n = 5 (5$\times$5 patch) & 27.41 & 0.77 & 0.153 \\
        \hline
    \end{tabular}
}
\caption{The impact of the local patch size n on different performance metrics. The results are evaluated on the DIV2K validation set with temperature $\tau=0.6$.}
\label{tab:supp:patch_size}
\end{table}
We demonstrate the effect of a larger patch size in Table~\ref{tab:supp:patch_size}. A larger patch size ($n=5$) achieves better LPIPS than the smaller one ($n=3$) while having comparable PSNR and SSIM, proving that a larger patch can better capture the underlying distribution and generate rich and reasonable texture details. Moreover, we observe that while $3 \times 3$ patch brings a substantial improvement in LPIPS compared to pixel-based model, $5 \times 5$ patch brings a relatively small improvement compared to $3 \times 3$ patch. The insight of this observation is the locality of textural details in natural images. Since texture details are locally correlated, a small patch size is sufficient to capture the distribution of local texture details. Therefore, the improvements are likely to saturate as patch size increases. A Similar observation has been found in~\cite{larsr}.

\subsection{Generative SR Model in Arbitrary-Scale Setting} 
\label{subsec:generative_arbit}
\begin{table}[t]

\newcommand{\mytoprule}{\toprule[1.2pt]}
\centering
\footnotesize
\resizebox{\columnwidth}{!}{%
    \begin{tabular}{l|c|c|c|c}
        \hline
        \multirow{2}{*}{Method} & \multicolumn{4}{c}{Scale} \\ 
         & \multicolumn{1}{c}{x3} & \multicolumn{1}{c}{x3.25} & \multicolumn{1}{c}{x3.5} & \multicolumn{1}{c}{x3.75} \\ \hline \hline
         
        ESRGAN (+bicubic) \cite{esrgan} & 28.94 / 0.076 & 28.37 / 0.087 & 27.85 / 0.097 & 27.39 / 0.107 \\
        
        RankSRGAN (+bicubic) \cite{ranksrgan} & 28.63 / 0.087 & 28.09 / 0.097 & 27.61 / 0.108 & 27.19 / 0.118 \\
        
        SRFlow (+bicubic) $\tau$ = 0.9 \cite{srflow} & 29.33 / 0.082 & 28.77 / 0.092 & \textbf{28.26} / 0.103 & \textbf{27.77} / 0.113 \\ 
        
        HCFlow (+bicubic) $\tau$ = 0.9 \cite{hcflow} & 28.88 / 0.072 & 28.32 / 0.082 & 27.81 / 0.092 & 27.36 / 0.102 \\
        
        \textbf{Ours} $\tau$ = 0.8 & \textbf{29.44} / \textbf{0.069} & \textbf{28.79} / \textbf{0.080} & 28.24 / \textbf{0.090} & 27.76 / \textbf{0.101}  \\
        \hline

    \end{tabular}
}
\caption{The arbitrary-scale SR results  (PSNR / LPIPS) evaluated on the DIV2K validation set, where the values of PSNR are evaluated on the RGB space. (+bicubic) means that the model first generates $\times$4 HR image and then down-scale to the specified scale using bicubic interpolation.}
\label{tab:exp:generative_on_arbitrary}
\end{table}
We follow the same evaluation strategy adopted in Meta-SR~\cite{metasr} to evaluate the performance of generative SR models in the arbitrary-scale SR setting. Specifically, given an arbitrary scale $s$ and an LR image, we first generate an $\times$4 HR image for those fixed-scale $\times$4 generative SR models \cite{esrgan, ranksrgan, srflow, hcflow}. Then, we down-scale the $\times$4 HR image with scaling factor $s/4$ with bicubic interpolation to produce the final HR image. In this experiment, all models use the same backbone~\cite{esrgan} and trained on the same datasets~\cite{div2k, flickr2k}. Our LINF adopts the proposed patch-based method with $n = 3$. Table~\ref{tab:exp:generative_on_arbitrary} presents a quantitative comparison of LINF and several fixed-scale SR methods for arbitrary-scale SR, where the performance is evaluated based on four different scales: $\times$3, $\times$3.25, $\times$3.5 and $\times$3.75. We can observe that as the scale moves away from $\times$4, the performance of the fixed-scale SR methods drop, allowing LINF to surpass them by noticeable margins.
% LINF performs better than fixed-scale SR methods with an increasing performance gap. 
The performance gap is caused by the fact that the images generated by fixed-scale SR model have to undergo a down-scaling process, leading to degraded qualities. In contrast, LINF directly generates SR images according to the specified scale without the need of the down-scaling process, allowing it to preserve the qualities of the generated images more precisely.

The experimental evidence thus validates that the proposed LINF is indeed able to generalize to arbitrary-scale SR better than those fixed-scale SR methods. It also validates the necessity of arbitrary-scale SR framework on SR tasks because this framework avoids blurry images caused by post-processing.

\begin{table*}[t]

\newcommand{\mytoprule}{\toprule[1.2pt]}
\centering
\footnotesize
\setlength{\tabcolsep}{1.5em}
\resizebox{1.8\columnwidth}{!}{%
    \begin{tabular}{c|l}
        \mytoprule
        Symbol & Description  \\
        \mytoprule
        $n$ & Patch size of our LINF model. \\
        $I^{LR}$ & Low Resolution image. \\
        $I^{HR}$ & High Resolution image. \\
        $I^{LR}_{\uparrow}$ & Bilinearly upsampled Low Resolution image. \\
        $I^{HR}_{texture}$ & Texture of High Resolution image, defined as the residual between $I^{HR}$ and $I^{LR}_{\uparrow}$. \\
        $s$ & Upscaling factor. \\
        $m_{i,j}$ & Local texture patch with index $(i, j)$. \\
        $x_{i,j}$ & Coordinate of local texture patch $m_{i,j}$. \\
        \hline
        $f_{\theta}$ & Normalizing Flow model with parameter $\theta$. \\
        $z$ & Latent variable with Gaussian distribution. \\
        $h$ & Intermediate latent variable in the flow transformation. \\
        $\tau$ & Temperature of Gaussian distribution, i.e, variance. \\
        \hline
        $E_{\Psi}$ & Local Texture Estimator with parameter $\Psi$.\\
        $g_{\Phi}$ & Parameter Generator with parameter $\Phi$.\\
        $c$ & Cell size, calculated as $c=2/s$. \\
        $v$ & Feature vector of Low Resolution image. \\
        $\Upsilon$ & The set of four nearest feature vectors given a query coordinate $x_q$. \\
        $w$ & Ensemble weight of bilinear interpolation. \\
        \mytoprule
    \end{tabular}
}
\caption{A list of the symbols used in this paper.}
\label{tab:supp:notation}
\end{table*}

\section{Additional Qualitative Results}
\label{sec::qualitative}
In this section, we present more qualitative results in Figs.~\ref{fig:supp_1} and~\ref{fig:supp_2}. The qualitative results show that LINF is indeed able to generate photo-realistic HR images, which are better in visual quality than the overly smoothed ones generated by LTE\cite{lte}.
% The results demonstrate that LINF can indeed generate photo-realistic HR images compared to the over-smoothed ones generated by LTE\cite{lte}.

\begin{figure*}[t]
  \centering
  \includegraphics[width=0.8\linewidth]{images/arbit_1.pdf}
  \caption{
    Qualitative comparisons on arbitrary-scale SR, we evaluated on DIV2K validation set with 4.3$\times$ SR. Images on the left are generated by LTE~\cite{lte}, and the right ones are generated by our LINF. 
  }
  \label{fig:supp_1}
\end{figure*}

\begin{figure*}[t]
  \centering
  \includegraphics[width=0.8\linewidth]{images/arbit_2.pdf}
  \caption{
    Qualitative comparisons on arbitrary-scale SR, we evaluated on DIV2K validation set with 4.3$\times$ SR. Images on the left are generated by LTE~\cite{lte}, and the right ones are generated by our LINF. 
  }
  \label{fig:supp_2}
\end{figure*}
