# Supplementary material for: Local Implicit Normalizing Flow for Arbitrary-Scale Image Super-Resolution
Source: arXiv:2303.05156 source file (2023-07-13)
Supplement: Supplementary file 2 [file background.tex]

% \subsection{Normalizing Flow} 
% \label{subsec:nf}

% In this section, we introduce background knowledge of implicit neural representation to make our paper self-contained.
In this section, we briefly review the essential background knowledge of implicit neural representation to allow the presentation of this work self-contained.

\subsection{Implicit Neural Representation} 
\label{subsec:inr}
Implicit neural representation parametrized by multilayer perceptron (MLP) approximates complex signals by mapping input coordinates to output values. Compared to classic discrete representation (e.g., pixels for 2D images and point clouds, meshes, and voxel grids for 3D objects), Such coordinate-based MLP successfully represents the signals in the continuous domain. Recent works have achieved promising results in modeling 2D images~\cite{siren, liif} and 3D geometry and appearance~\cite{imnet, Occupancy_Networks, deepsdf, srn, nerf}.
However, many previous works focus on fitting the signal of a single instance, e.g., an image~\cite{siren} or a scene~\cite{nerf}. To make implicit neural representation generalize to unseen data, latent vector conditioning~\cite{Occupancy_Networks, deepsdf} and hypernetwork setting~\cite{srn, siren} have been proposed. The former fed the latent vector corresponding to a particular instance along with coordinates to the MLP network, and the latter used a hypernetwork to map a latent to the weights of MLP. 
Our work is based on the idea of local implicit neural representation~\cite{jiang2020lig, liif}. Instead of taking a global latent as a condition, local implicit neural representation captures the localized details by conditioning on a local feature.
