# Supplementary material for: Local Implicit Normalizing Flow for Arbitrary-Scale Image Super-Resolution
Source: arXiv:2303.05156 source file (2023-07-13)
Supplement: Supplementary file 3 [file experiment.tex]

\subsection{Analysis on the Patch Size} 
\label{subsec:patch}
\begin{table}[t]

\centering
\footnotesize
\resizebox{0.8\columnwidth}{!}{%
    \begin{tabular}{l|c|c|c}
        \hline
        Method & PSNR$\uparrow$ & SSIM$\uparrow$ & LPIPS$\downarrow$ \\
        \hline
        \hline
        n = 1 (pixel) & 27.94 & 0.79 & 0.174 \\
        n = 3 (3$\times$3 patch) & 27.43 & 0.77 & 0.158 \\
        n = 5 (5$\times$5 patch) & 27.41 & 0.77 & 0.153 \\
        \hline
    \end{tabular}
}
\caption{The impact of the local patch size n on different performance metrics. The results are evaluated on the DIV2K validation set with temperature $\tau=0.6$.}
\label{tab:supp:patch_size}
\end{table}
We demonstrate the effect of a larger patch size in Table~\ref{tab:supp:patch_size}. A larger patch size ($n=5$) achieves better LPIPS than the smaller one ($n=3$) while having comparable PSNR and SSIM, proving that a larger patch can better capture the underlying distribution and generate rich and reasonable texture details. Moreover, we observe that while $3 \times 3$ patch brings a substantial improvement in LPIPS compared to pixel-based model, $5 \times 5$ patch brings a relatively small improvement compared to $3 \times 3$ patch. The insight of this observation is the locality of textural details in natural images. Since texture details are locally correlated, a small patch size is sufficient to capture the distribution of local texture details. Therefore, the improvements are likely to saturate as patch size increases. A Similar observation has been found in~\cite{larsr}.

\subsection{Generative SR Model in Arbitrary-Scale Setting} 
\label{subsec:generative_arbit}
\begin{table}[t]

\centering
\footnotesize
\resizebox{\columnwidth}{!}{%
    \begin{tabular}{l|c|c|c|c}
        \hline
        \multirow{2}{*}{Method} & \multicolumn{4}{c}{Scale} \\ 
         & \multicolumn{1}{c}{x3} & \multicolumn{1}{c}{x3.25} & \multicolumn{1}{c}{x3.5} & \multicolumn{1}{c}{x3.75} \\ \hline \hline
         
        ESRGAN (+bicubic) \cite{esrgan} & 28.94 / 0.076 & 28.37 / 0.087 & 27.85 / 0.097 & 27.39 / 0.107 \\
        
        RankSRGAN (+bicubic) \cite{ranksrgan} & 28.63 / 0.087 & 28.09 / 0.097 & 27.61 / 0.108 & 27.19 / 0.118 \\
        
        SRFlow (+bicubic) $\tau$ = 0.9 \cite{srflow} & 29.33 / 0.082 & 28.77 / 0.092 & \textbf{28.26} / 0.103 & \textbf{27.77} / 0.113 \\ 
        
        HCFlow (+bicubic) $\tau$ = 0.9 \cite{hcflow} & 28.88 / 0.072 & 28.32 / 0.082 & 27.81 / 0.092 & 27.36 / 0.102 \\
        
        \textbf{Ours} $\tau$ = 0.8 & \textbf{29.44} / \textbf{0.069} & \textbf{28.79} / \textbf{0.080} & 28.24 / \textbf{0.090} & 27.76 / \textbf{0.101}  \\
        \hline

    \end{tabular}
}
\caption{The arbitrary-scale SR results  (PSNR / LPIPS) evaluated on the DIV2K validation set, where the values of PSNR are evaluated on the RGB space. (+bicubic) means that the model first generates $\times$4 HR image and then down-scale to the specified scale using bicubic interpolation.}
\label{tab:exp:generative_on_arbitrary}
\end{table}
We follow the same evaluation strategy adopted in Meta-SR~\cite{metasr} to evaluate the performance of generative SR models in the arbitrary-scale SR setting. Specifically, given an arbitrary scale $s$ and an LR image, we first generate an $\times$4 HR image for those fixed-scale $\times$4 generative SR models \cite{esrgan, ranksrgan, srflow, hcflow}. Then, we down-scale the $\times$4 HR image with scaling factor $s/4$ with bicubic interpolation to produce the final HR image. In this experiment, all models use the same backbone~\cite{esrgan} and trained on the same datasets~\cite{div2k, flickr2k}. Our LINF adopts the proposed patch-based method with $n = 3$. Table~\ref{tab:exp:generative_on_arbitrary} presents a quantitative comparison of LINF and several fixed-scale SR methods for arbitrary-scale SR, where the performance is evaluated based on four different scales: $\times$3, $\times$3.25, $\times$3.5 and $\times$3.75. We can observe that as the scale moves away from $\times$4, the performance of the fixed-scale SR methods drop, allowing LINF to surpass them by noticeable margins.
% LINF performs better than fixed-scale SR methods with an increasing performance gap. 
The performance gap is caused by the fact that the images generated by fixed-scale SR model have to undergo a down-scaling process, leading to degraded qualities. In contrast, LINF directly generates SR images according to the specified scale without the need of the down-scaling process, allowing it to preserve the qualities of the generated images more precisely.

The experimental evidence thus validates that the proposed LINF is indeed able to generalize to arbitrary-scale SR better than those fixed-scale SR methods. It also validates the necessity of arbitrary-scale SR framework on SR tasks because this framework avoids blurry images caused by post-processing.
