# Supplementary material for: Local Implicit Normalizing Flow for Arbitrary-Scale Image Super-Resolution
Source: arXiv:2303.05156 source file (2023-07-13)
Supplement: Supplementary file 4 [file github.tex]

The anonymous GitHub link of our project:  \url{https://anonymous.4open.science/r/LINF-1674}
