# Supplementary material for: Local Implicit Normalizing Flow for Arbitrary-Scale Image Super-Resolution
Source: arXiv:2303.05156 source file (2023-07-13)
Supplement: Supplementary file 5 [file notation.tex]

The symbols used in this paper are summarized in Table~\ref{tab:supp:notation}.
