# Supplementary material for: Local Implicit Normalizing Flow for Arbitrary-Scale Image Super-Resolution
Source: arXiv:2303.05156 source file (2023-07-13)
Supplement: Supplementary file 6 [file qualitative.tex]

In this section, we present more qualitative results in Figs.~\ref{fig:supp_1} and~\ref{fig:supp_2}. The qualitative results show that LINF is indeed able to generate photo-realistic HR images, which are better in visual quality than the overly smoothed ones generated by LTE\cite{lte}.
% The results demonstrate that LINF can indeed generate photo-realistic HR images compared to the over-smoothed ones generated by LTE\cite{lte}.

\begin{figure*}[t]
  \centering
  \includegraphics[width=0.8\linewidth]{images/arbit_1.pdf}
  \caption{
    Qualitative comparisons on arbitrary-scale SR, we evaluated on DIV2K validation set with 4.3$\times$ SR. Images on the left are generated by LTE~\cite{lte}, and the right ones are generated by our LINF. 
  }
  \label{fig:supp_1}
\end{figure*}

\begin{figure*}[t]
  \centering
  \includegraphics[width=0.8\linewidth]{images/arbit_2.pdf}
  \caption{
    Qualitative comparisons on arbitrary-scale SR, we evaluated on DIV2K validation set with 4.3$\times$ SR. Images on the left are generated by LTE~\cite{lte}, and the right ones are generated by our LINF. 
  }
  \label{fig:supp_2}
\end{figure*}
